# Supplementary material for: Highly Efficient 3D Human Pose Tracking from Events with Spiking Spatiotemporal Transformer
Source: arXiv:2303.09681 source file (2025-05-15)
Supplement: Supplementary file 1 [file appendix.tex]

\appendices

\section{Spike-Element-Wise Residual Networks}
\label{sec:supp-sew-resnet}

SEW-ResNet, proposed in~\cite{fang2021deep}, is one of the most popular architectures of SNNs. It is largely based on ResNet~\cite{he2016deep}, but with significant differences in the design of the identity mapping for SNNs, where element-wise addition is applied to spike tensors rather than pre-spiking potentials. This design achieves accurate identity mapping of residual learning in SNNs, and also addresses the issue of vanishing and exploding gradients. Here it is used as the backbone in our pipeline to extract spike pose features. We show the detailed architecture of SEW-ResNet34~\cite{fang2021deep} in Fig.~\ref{fig:spiking-cnn}. There are also options of SEW-ResNet18, 50, 101 and 152 which have a similar architecture to SEW-ResNet34. The spatial size of the output is $1/32$ of the input with a channel size of $512$ for SEW-ResNet18, 34 and $2048$ for SEW-ResNet50, 101, 152.

SEW-ResNet consists of two types of blocks: the downsample block and the basic block. The downsample block normally reduces the spatial size of input spike tensor by 2 and expands the channel size by 4 through convolutional layers, while the basic block keeps the size of input spike tensor unchanged for residual learning. The final layer in both types of blocks is element-wise identity mapping via \textit{SEW Function}, where spike-element-wise functions between two input spike tensors are applied, such as ADD, AND or IAND. Given the input spike tensor $\mathbf{S}^{\text{in}}\in \{0, 1\}^{T\times H\times W\times C^{\text{in}}}$, the output spike tensor is assumed to be $\mathbf{S}^{\text{out}}\in \{0, 1\}^{T\times \frac{H}{32}\times \frac{W}{32}\times C}$ where $C=512$ for SEW-ResNet18 and 34, $C=2048$ for SEW-ResNet50, 101 and 152.

\begin{figure}[h!]
    \centering
    \includegraphics[width=\columnwidth]{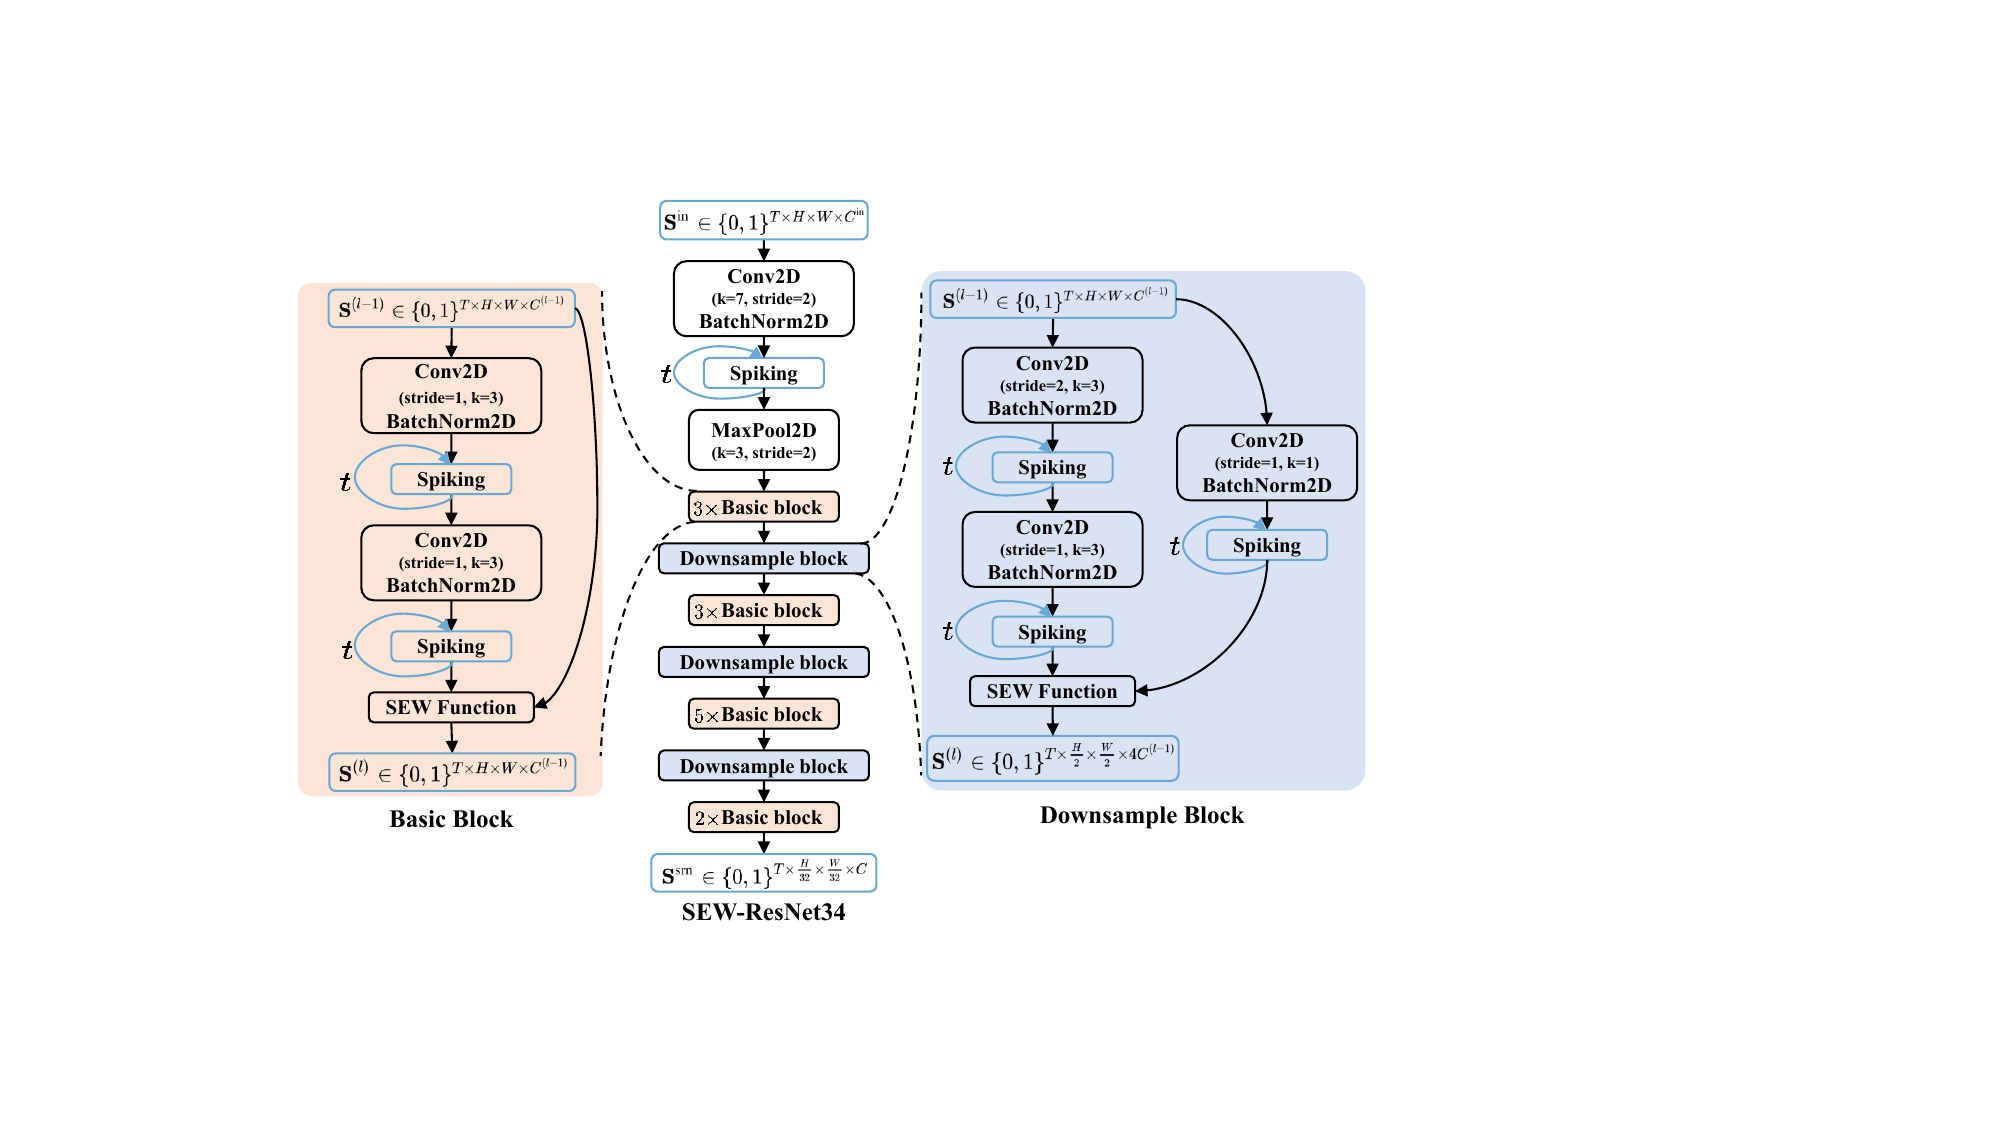}
    \caption{\textbf{Architecture of SEW-ResNet34.} Given the input spike tensor $\scriptstyle \mathbf{S}^{\text{in}}\in \{0, 1\}^{T\times H\times W\times C}$, the output spike tensor is $\scriptstyle \mathbf{S}^{\text{out}}\in \{0, 1\}^{T\times \frac{H}{32}\times \frac{W}{32}\times C}$ where $\scriptstyle C=512$ for SEW-ResNet34. SEW-ResNet is comprised of two types of blocks: the downsample block and the basic block. The downsample block reduces the spatial size of the input spike tensor by 2 and increases the channel size by 4 through convolutional layers, while the basic block maintains the size of the input spike tensor for residual learning in SNNs. The final layer in both types of blocks is element-wise identity mapping via \textit{SEW Function}, where spike-element-wise functions between two input spike tensors are applied, such as ADD, AND or IAND.}
    \label{fig:spiking-cnn}
\end{figure}

\section{Proof of Proposition 1}
\label{sec:supp-proof}
\begin{lemma}[Johnson–Lindenstrauss Lemma on Binary Embedding~\cite{jacques2013robust,yi2015binary}]
\label{lemma:JL-Lemma}
Let $\{\mathbf{x}_i\}_{i=1}^{M}$ be set of $M$ real-valued points, define its one bit quantization of the projections,
\begin{equation}
    \mathbf{s}(\mathbf{x}) = \text{sign}(\mathbf{Ax}), 
\end{equation}
where $\mathbf{s}(\mathbf{x})\in \{0, 1\}^{C_k}$ is the binary embedding of $\mathbf{x}\in\mathbb{R}^{d_k}$ and $\mathbf{A}\in \mathbb{R}^{C_k\times d_k}$ is a projection matrix with each entry generated independently from the normal distribution $\mathcal{N}(0, 1)$. Given $\scriptstyle C_k > \frac{\log M}{\delta^2}$, for any two points among $M$, 
\begin{equation}
    \label{eq:equivalency}
    |f_{\mathcal{H}}(\mathbf{s}_i, \mathbf{s}_j) - f_{\mathcal{C}}(\mathbf{x}_i, \mathbf{x}_j)| \leq \delta
\end{equation}
holds true with probability at least $1-2e^{-\delta^2 C_k}$. Here $f_{\mathcal{H}}$ is the normalized Hamming distance defined as
\begin{equation}
    \label{eq:hamming-distance}
    f_{\mathcal{H}}(\mathbf{s}_i, \mathbf{s}_j) = \frac{1}{C_k}\sum_{k=1}^{C_k} \mathds{1}(\mathbf{s}_{ik} \neq \mathbf{s}_{jk}),
\end{equation}
and $f_{\mathcal{C}}$ is cosine distance defined as
\begin{equation}
    \label{eq:cosine-distance}
    f_{\mathcal{C}}(\mathbf{x}_i, \mathbf{x}_j) = \frac{1}{\pi} \arccos \Big( \frac{\mathbf{x}_i^{\top}\mathbf{x}_j}{\|\mathbf{x}_i\|\|\mathbf{x}_j\|}\Big).
\end{equation}
\end{lemma}

According to Lemma~\ref{lemma:JL-Lemma}, we have the proof of Proposition~\ref{proposition:hamming-similarity} as follows:
\begin{proof}
By substituting $\mathbf{x}_i, \mathbf{x}_j, \mathbf{s}_i, \mathbf{s}_j$ in Eq.~(\ref{eq:equivalency}) with $\mathbf{q}_i, \mathbf{k}_j, \mathbf{s}_i^q, \mathbf{s}_j^k$ respectively, we have
\begin{equation}
    \begin{aligned}
        f_{\mathcal{H}}(\mathbf{s}_i^q, \mathbf{s}_j^k) - \delta \leq f_{\mathcal{C}}(\mathbf{q}_i, \mathbf{k}_j) \leq f_{\mathcal{H}}(\mathbf{s}_i^q, \mathbf{s}_j^k) + \delta. \\
    \end{aligned}
\end{equation}
After replacing $f_{\mathcal{H}}, f_{\mathcal{C}}$ defined in Eq.~(\ref{eq:hamming-distance}) and~(\ref{eq:cosine-distance}) with $d_{\mathcal{H}}, d_{\mathcal{C}}$ defined in Eq.~(\ref{eq:hamming-similarity}) and~(\ref{eq:cosine-similarity}), we have 
\begin{equation}\footnotesize
    \begin{aligned}
        & 1-d_{\mathcal{H}}(\mathbf{s}_i^q, \mathbf{s}_j^k) - \delta \leq \frac{1}{\pi} \arccos \Big(d_{\mathcal{C}}(\mathbf{q}_i, \mathbf{k}_j) \Big) \leq 1-d_{\mathcal{H}}(\mathbf{s}_i^q, \mathbf{s}_j^k) + \delta, \\
        & \cos\Big(\pi\big(1-d_{\mathcal{H}}(\mathbf{s}^q_i, \mathbf{s}^k_j) + \delta\big)\Big)\leq d_{\mathcal{C}}(\mathbf{q}_i, \mathbf{k}_j) \leq \cos\Big(\pi\big(1-d_{\mathcal{H}} (\mathbf{s}^q_i, \mathbf{s}^k_j) - \delta\big)\Big). 
    \end{aligned}
\end{equation}
Define the function $g(x)=\cos(\pi(1-x))$, we have
\begin{equation}
    g(d_{\mathcal{H}}(\mathbf{s}^q_i, \mathbf{s}^k_j) - \delta) \leq d_{\mathcal{C}}(\mathbf{q}_i, \mathbf{k}_j) \leq g(d_{\mathcal{H}}(\mathbf{s}^q_i, \mathbf{s}^k_j) + \delta).
\end{equation}
\end{proof}

\section{SynEventHPD Dataset}
\label{sec:supp-dataset}
\textbf{The synthesizing process} of our proposed dataset is mainly based on the workflow proposed in~\cite{gehrig2020video}. Given an RGB video, we first detect the bounding box of the person in each frame using 2D pose annotations or 2D pose detector like OpenPose~\cite{cao2019openpose}. After calculating the global bounding box of the person in the video, we crop it accordingly and resize to $512\times 512$ to maintain a same image size across different sub-datasets. Next, we apply the approach proposed in~\cite{jiang2018super} for frame interpolation guided by the predicted optical flows to increase the frame rate of provided videos. After converting the high frame rate RGB videos to gray-scale images, we generate events by checking the brightness change at each pixel over time, where the contrast thresholds for positive and negative events are $0.3$ and the minimum waiting period before a pixel can trigger a new event is 1e-4 seconds. This process is straightforward for Human3.6M~\cite{ionescu2013human3}, PHSPD~\cite{zou2022human} and MMHPSD~\cite{zou2021eventhpe}, as they contain RGB or gray-scale videos. We name the three sub-datasets as EventH36M, EventPHSPD and SynMMHPSD respectively. Since the three datasets provide corresponding SMPL pose and shape annotations, we keep them in our dataset while calculating an optimal global translation for each frame by aligning projected 3D poses with annotated 2D poses on the image, using the default camera intrinsic $(\text{focal\_length}, \text{center})=(671.72, 256.4)$. The FPS of pose annotations in EventPHSPD and SynMMHPSD is 15 while FPS in EventH36M is 10 based on the observations that the motions in Human3.6M are relatively slow.

AMASS~\cite{mahmood2019amass} dataset only contains motion capture data without any RGB videos. In this regard, for each motion capture sequence, an avatar is randomly picked from 13 different avatars shown in Fig.~\ref{fig:amass_avatars}, animated and rendered to form its corresponding RGB videos of size $512\times 512$, obtained using one of the 4 predefined lightning conditions displayed in Tab.~\ref{tab:light}. These 4 lightning conditions represent the positions of top center, left and right top, left and right bottom with different strength of illumination ranging from 0 to 1. To ensure the rendered avatar remains within the camera’s field of view, we appropriately adjust the trajectory (\ie, the global translations of each frame) of each sequence. By combining these adjusted global translations with the original SMPL pose and shape annotations, we generate new annotations for each sequence in AMASS. The following process of events generation is the same with the 3 sub-datasets mentioned above. We observe the FPS of AMASS motion sequences contains 60, 100 and 120. To make FPS of annotations across all the sequences, we downsample the FPS of motion to 20 before animation. Finally, we obtain the sub-dataset EventAMASS. We show a motion clip from each sub-dataset in Fig.~\ref{fig:dataset-example} to further illustrate the efficacy of our synthetic events.

\begin{table}[h!]
    \centering
    \caption{Four predefined lightning conditions used for rendering in EventAMASS dataset.}
    \setlength{\tabcolsep}{0.5mm}
    
    \resizebox{0.7\columnwidth}{!}{
    \begin{tabular}{@{}|c|c|@{}}
    \bottomrule \hline
        \makecell[c]{Lightning} & \makecell[c]{(Position, Color)} \\
    \hline
        1 & \makecell[c]{([0, 0, -300], [1.0, 1.0, 1.0])}\\
    \hline
        2 & \makecell[c]{([-300, -300, -300], [0.8, 0.8, 0.8])\\ ([300, -300, -300], [0.8, 0.8, 0.8])} \\
    \hline
        3 & \makecell[c]{([300, 0, -300], [1, 1, 1]) \\ ([-300, 0, -300], [0.4, 0.4, 0.4])} \\
    \hline
        4 & \makecell[c]{([300, 0, -300], [0.4, 0.4, 0.4]) \\ ([-300, 0, -300], [1, 1, 1])} \\
    \hline \toprule 
    \end{tabular}}
    \label{tab:light}
\end{table}

\begin{figure*}[h!]
    \centering
    \includegraphics[width=\textwidth]{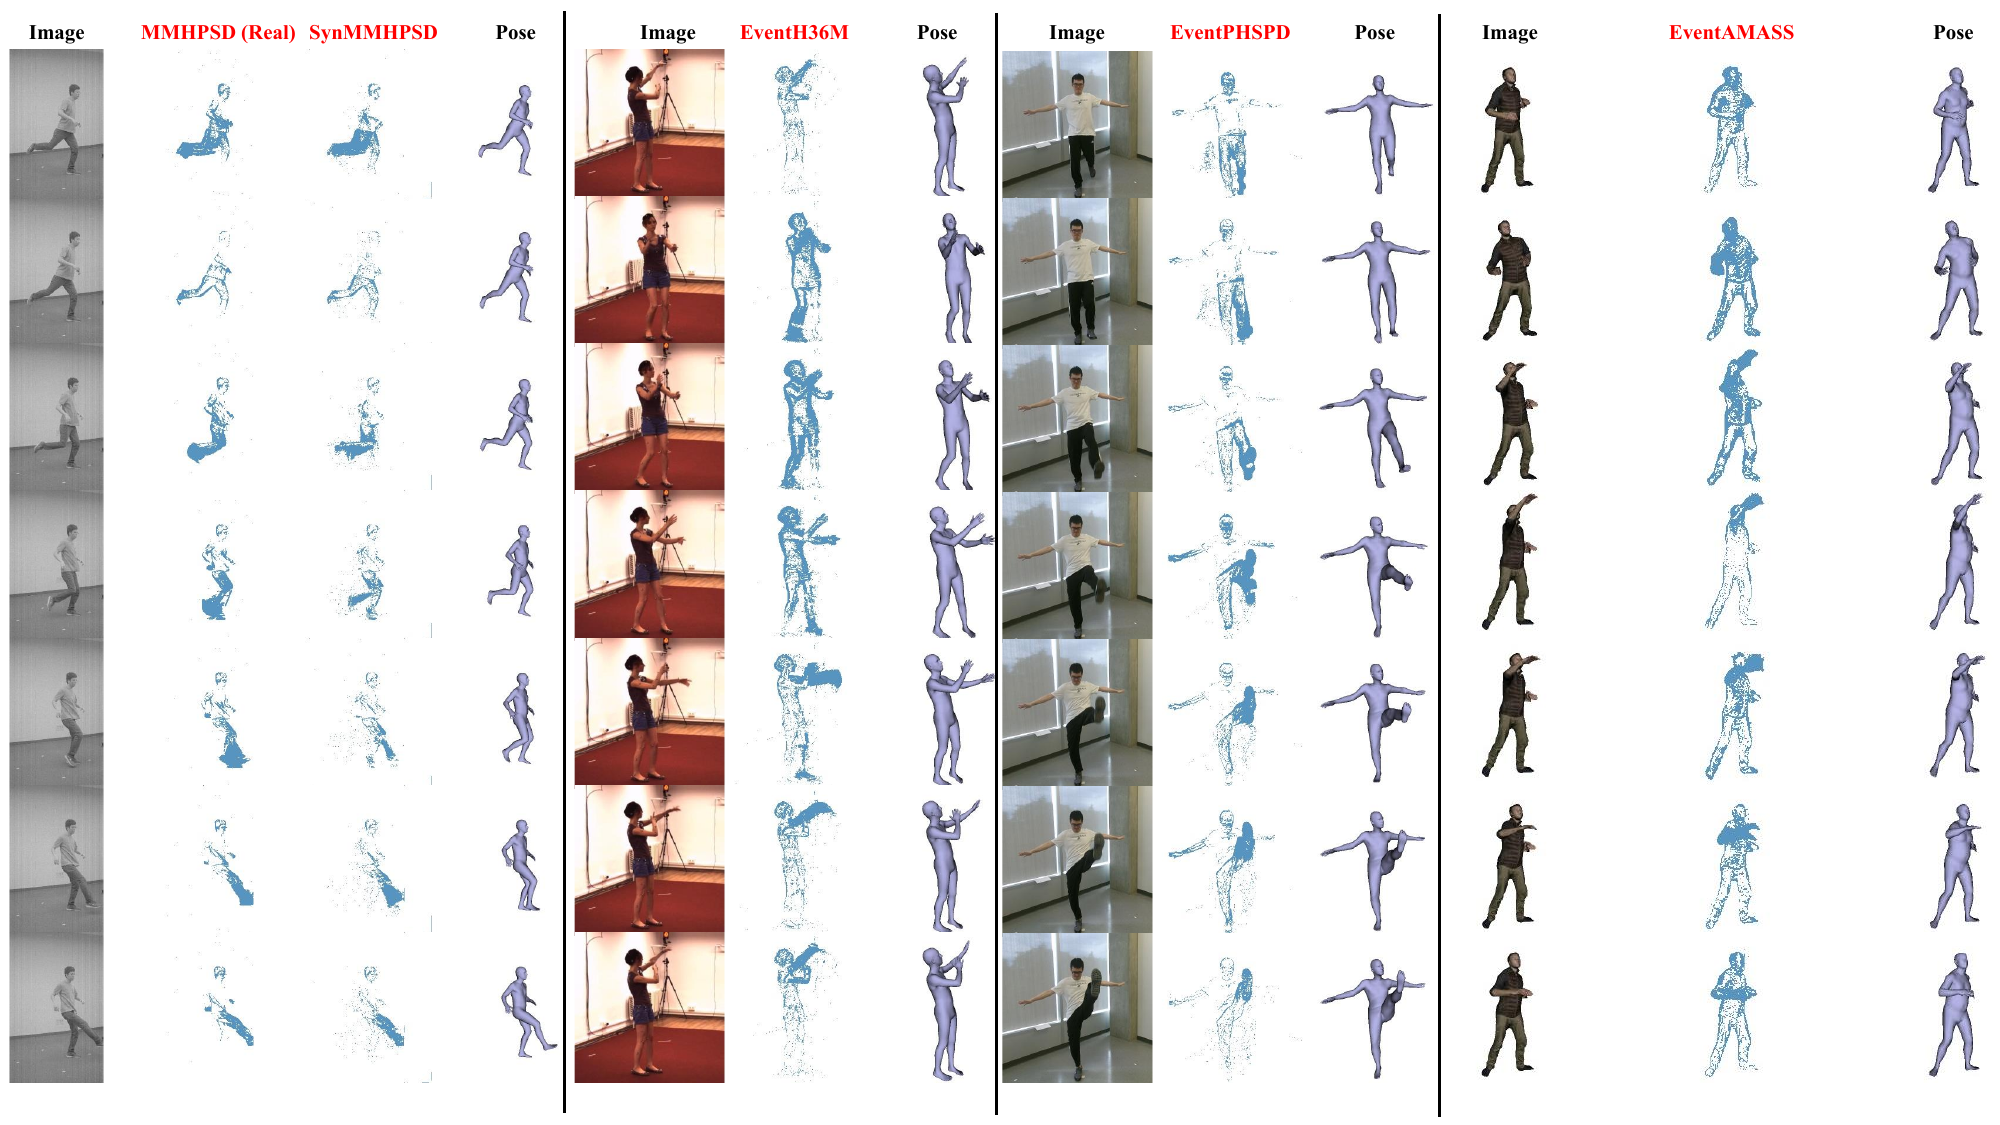}
    \caption{\textbf{Example Sequence} from Each Sub-Dataset in our SynEventHPD dataset.}
    \label{fig:dataset-example}
\end{figure*}

\begin{figure*}[h!]
    \centering
    \includegraphics[width=\textwidth]{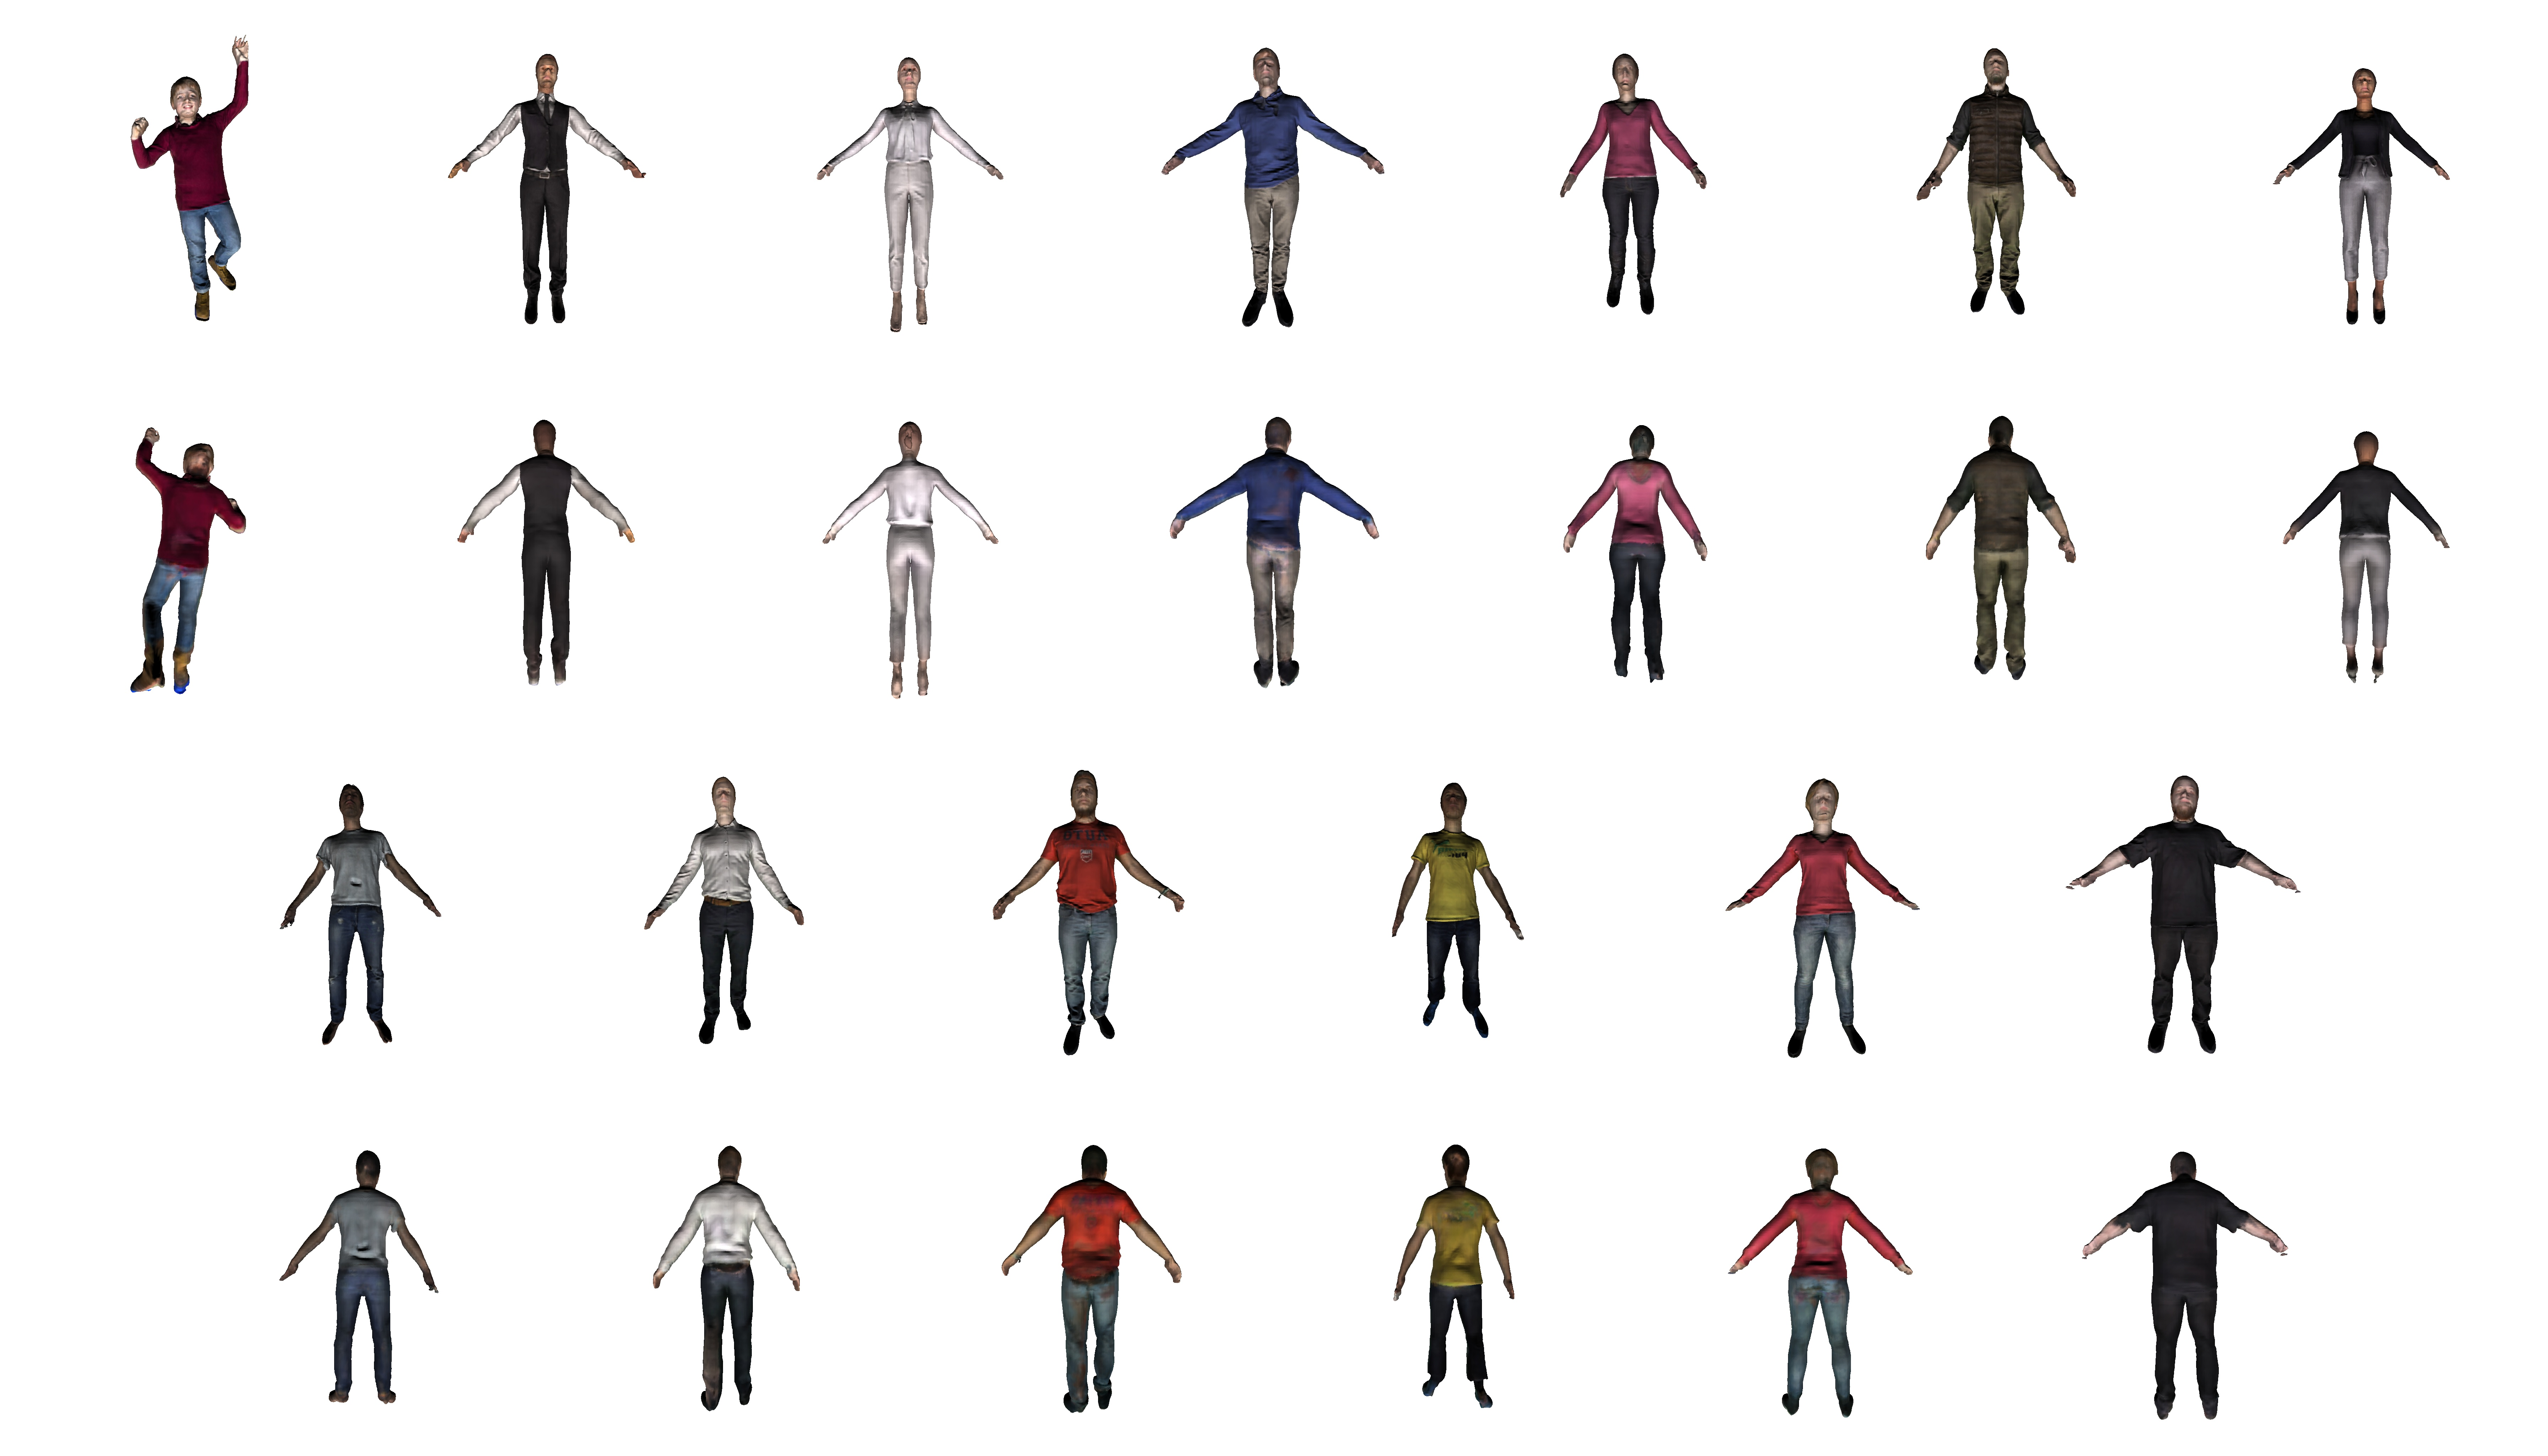}
    \caption{Front and Back Views of 13 Avatars used in EventAMASS dataset.}
    \label{fig:amass_avatars}
\end{figure*}

\section{Backpropagation in SNNs}
\label{sec:supp-backpropagation}
\textbf{Backpropagation through time in SNNs.} Given the backpropagated gradients from the last layer, $\frac{\partial \mathcal{L}}{\mathbf{s}^{(l)}_{[t]}}$, we can unfold the iterative update of membrane potential for $T$ time steps and calculate the gradients $\frac{\partial \mathcal{L}}{\partial \mathbf{s}^{(l-1)}_{[t]}}$ and $\frac{\partial \mathcal{L}}{\partial \mathbf{W}^{(l)}}$ respectively. As is analysed in~\cite{xiao2022online}, the derivative of the Heaviside step function is 0 almost everywhere, allowing us to detach the neuron reset operation from the computational graph and avoid backpropagating gradients along this path. So we have the BPTT in SNNs shown in Fig.~\ref{fig:neuron_model}~(c). The detailed derivatives are provided below.
\clearpage
\begin{strip}
Considering only $\mathbf{s}^{(l)}_{[k]}$ ($k \geq t$) depends on $\mathbf{s}^{(l-1)}_{[t]}$, the loss function can be described as
\begin{equation}
\begin{aligned}
    \mathcal{L}
    \bigg(
        \mathbf{s}^{(l)}_{[t]}
        \Big(
            \begingroup \color{orange} \mathbf{h}^{(l)}_{[t]}
            \big(
                \mathbf{s}^{(l-1)}_{[t]}
            \big) \endgroup
        \Big),\quad
        \mathbf{s}^{(l)}_{[t+1]}
        \Big(
            \mathbf{h}^{(l)}_{[t+1]}
            \Big(
                \begingroup \color{blue} \mathbf{h}^{(l)}_{[t]}(\mathbf{s}^{(l-1)}_{[t]}) \endgroup,
                \mathbf{s}^{(l)}_{[t]}(
                    \begingroup \color{pink} \mathbf{h}^{(l)}_{[t]}(\mathbf{s}^{(l-1)}_{[t]}) \endgroup
                )
            \Big)
        \Big),\quad
        \mathbf{s}^{(l)}_{[t+2]}
            \Big(
                ...
            \Big),
        ...
    \bigg) 
    .
\end{aligned}
\end{equation}
Then we have the gradient of loss with respect to $\mathbf{s}^{(l-1)}_{[t]}$ from layer $l$ to layer $l-1$ as
\begin{equation}
\begin{aligned}
    \frac{\partial \mathcal{L}}{\partial \mathbf{s}^{(l-1)}_{[t]}} &= 
    % first term
    \frac{\partial \mathcal{L}}{\partial \mathbf{s}^{(l)}_{[t]}}
    \frac{\partial \mathbf{s}^{(l)}_{[t]}}{\partial \mathbf{h}^{(l)}_{[t]}}
    \begingroup \color{orange} \frac{\partial \mathbf{h}^{(l)}_{[t]}}{\partial \mathbf{s}^{(l-1)}_{[t]}} \endgroup + 
    % second term
    \frac{\partial \mathcal{L}}{\partial \mathbf{s}^{(l)}_{[t+1]}}
    \frac{\partial \mathbf{s}^{(l)}_{[t+1]}}{\partial \mathbf{h}^{(l)}_{[t+1]}} 
    \bigg(
        \underbrace{
            \frac{\partial \mathbf{h}^{(l)}_{[t+1]}}{\partial \mathbf{u}^{(l)}_{[t]}}
            \frac{\partial \mathbf{u}^{(l)}_{[t]}}{\partial \mathbf{h}^{(l)}_{[t]}}
        }_{\text{leak path}}
        \begingroup \color{blue} \frac{\partial \mathbf{h}^{(l)}_{[t]}}{\partial \mathbf{s}^{(l-1)}_{[t]}} \endgroup
        + 
        \underbrace{
            \frac{\partial \mathbf{h}^{(l)}_{[t+1]}}{\partial \mathbf{u}^{(l)}_{[t]}}
            \frac{\partial \mathbf{u}^{(l)}_{[t]}}{\partial \mathbf{s}^{(l)}_{[t]}}
            \frac{\partial \mathbf{s}^{(l)}_{[t]}}{\partial \mathbf{h}^{(l)}_{[t]}}
        }_{\text{reset path}}
        \begingroup \color{pink}  \frac{\partial \mathbf{h}^{(l)}_{[t]}}{\partial \mathbf{s}^{(l-1)}_{[t]}} \endgroup
    \bigg)
    + \dots \\
    & = 
    % first term
    \frac{\partial \mathcal{L}}{\partial \mathbf{s}^{(l)}_{[t]}}
    \frac{\partial \mathbf{s}^{(l)}_{[t]}}{\partial \mathbf{h}^{(l)}_{[t]}}
    \frac{\partial \mathbf{h}^{(l)}_{[t]}}{\partial \mathbf{s}^{(l-1)}_{[t]}} +
    % second term
    \frac{\partial \mathcal{L}}{\partial \mathbf{s}^{(l)}_{[t+1]}}
    \frac{\partial \mathbf{s}^{(l)}_{[t+1]}}{\partial \mathbf{h}^{(l)}_{[t+1]}} 
    \bigg(
        \underbrace{\lambda}_{\text{leak path}}
        - 
        \underbrace{
            V_{\text{th}}\frac{\partial \mathbf{s}^{(l)}_{[t]}}{\partial \mathbf{h}^{(l)}_{[t]}}
        }_{\text{reset path}}
    \bigg)
    \frac{\partial \mathbf{h}^{(l)}_{[t]}}{\partial \mathbf{s}^{(l-1)}_{[t]}}
    +
    \dots \\
    &= \sum_{k=t}^{T} 
    \underbrace{\frac{\partial \mathcal{L}}{\partial \mathbf{s}^{(l)}_{[k]}}}_{\substack{\text{gradient from} \\ \text{last layer}}}
    \underbrace{\frac{\partial \mathbf{s}^{(l)}_{[k]}}{\partial \mathbf{h}^{(l)}_{[k]}}}_{\substack{\text{surrogate} \\ \text{gradient}}}
    \Big( \mathbf{1} + 
        \prod_{\tau=t-1}^{k-1} 
        \big( 
            \lambda - V_{\text{th}}\underbrace{\frac{\partial \mathbf{s}^{(l)}_{[\tau]}}{\partial \mathbf{h}^{(l)}_{[\tau]}}}_{\substack{\text{surrogate} \\ \text{gradient}}}
        \big)
    \Big)
    \mathbf{W}^{(l)} \\
    & \overset{\substack{\text{detach} \\ \text{reset}}}{\approx} \sum_{k=t}^{T} 
    \lambda^{k-t}
    \frac{\partial \mathcal{L}}{\partial \mathbf{s}^{(l)}_{[k]}}
    \frac{\partial \mathbf{s}^{(l)}_{[k]}}{\partial \mathbf{h}^{(l)}_{[k]}}
    \mathbf{W}^{(l)}  .
\end{aligned}
\end{equation}
The loss at time step $t$ only depends on $\mathbf{h}^{(l)}_{[k]}$ where $k\leq t$,
\begin{equation}
\begin{aligned}
    \mathcal{L}_{t} \Big( 
    \mathbf{h}^{(l)}_{[t]}
    \Big) & = \mathcal{L}_{t} \Bigg( 
    \begingroup \color{orange} \mathbf{h}^{(l)}_{[t]} 
        \bigg( 
            \mathbf{W}^{(l)} \endgroup, 
            \mathbf{u}_{[t-1]}^{(l)}
    \begingroup \color{orange} \bigg) \endgroup
    \Bigg) \\
    & = \mathcal{L}_{t} \Bigg( 
    \begingroup \color{orange} \mathbf{h}^{(l)}_{[t]} 
        \bigg( \endgroup
            \underbrace{\begingroup \color{orange} \mathbf{W}^{(l)}\endgroup}_{\text{charge path}} ,\quad
            \mathbf{u}_{[t-1]}^{(l)}
            \Big(
                \underbrace{\begingroup \color{blue} \mathbf{h}_{[t-1]}^{(l)} 
                    \big( 
                        \mathbf{W}^{(l)}
                    \big)\endgroup }_{\text{leak path}} , \ 
                \underbrace{\mathbf{s}_{[t-1]}^{(l)}
                    \big(
                        \begingroup \color{pink} \mathbf{h}_{[t-1]}^{(l)} (\mathbf{W}^{(l)}) \endgroup
                    \big)}_{\text{spike and reset path}}
            \Big)
        \begingroup \color{orange} \bigg) \endgroup
    \Bigg) 
    .
\end{aligned}
\end{equation}
So we have the unfolded gradients of $\frac{\partial \mathcal{L}}{\partial \mathbf{W}^{(l)}}$ as
\begin{equation}
\begin{aligned}
    \frac{\partial \mathcal{L}}{\partial \mathbf{W}^{(l)}} & = \sum_{t=0}^T \frac{\partial \mathcal{L}}{\partial \mathbf{W}^{(l)}} = \sum_{t=0}^T \frac{\partial \mathcal{L}}{\partial \mathbf{h}^{(l)}_{[t]}}
    \begingroup \color{orange} \frac{\partial \mathbf{h}^{(l)}_{[t]}}{\partial \mathbf{W}^{(l)}}\endgroup,  \\
    & = \sum_{t=0}^T 
    \frac{\partial \mathcal{L}}{\partial \mathbf{h}^{(l)}_{[t]}}
    % charge path
    \Big(
    \underbrace{
        \begingroup \color{orange} \frac{\partial \mathbf{h}^{(l)}_{[t]}}{\partial \mathbf{W}^{(l)}} \endgroup
    }_{\text{charge path}} + 
    % leak path
    \underbrace{
        \frac{\partial \mathbf{h}^{(l)}_{[t]}}{\partial \mathbf{u}^{(l)}_{[t-1]}}
        \frac{\partial \mathbf{u}^{(l)}_{[t-1]}}{\partial \mathbf{h}^{(l)}_{[t-1]}}
        \begingroup \color{blue} \frac{\partial \mathbf{h}^{(l)}_{[t-1]}}{\partial \mathbf{W}^{(l)}} \endgroup
    }_{\text{leak path}} +
    % reset path
    \underbrace{
        \frac{\partial \mathbf{h}^{(l)}_{[t]}}{\partial \mathbf{u}^{(l)}_{[t-1]}}
        \frac{\partial \mathbf{u}^{(l)}_{[t-1]}}{\partial \mathbf{s}^{(l)}_{[t-1]}}
        \frac{\partial \mathbf{s}^{(l)}_{[t-1]}}{\partial \mathbf{h}^{(l)}_{[t-1]}}
        \begingroup \color{pink} \frac{\partial \mathbf{h}^{(l)}_{[t-1]}}{\partial \mathbf{W}^{(l)}} \endgroup
    }_{\text{spike and reset path}}
    \Big)
    ,  \\
    & = \sum_{t=0}^T 
    \frac{\partial \mathcal{L}}{\partial \mathbf{h}^{(l)}_{[t]}} 
    \Big( 
        \mathbf{s}^{(l)}_{[t]} + 
        \lambda \frac{\partial \mathbf{h}^{(l)}_{[t-1]}}{\partial \mathbf{W}^{(l)}} - 
        \lambda V_{\text{th}} \frac{\partial \mathbf{s}^{(l)}_{[t-1]}}{\partial \mathbf{h}^{(l)}_{[t-1]}}\frac{\partial \mathbf{h}^{(l)}_{[t-1]}}{\partial \mathbf{W}^{(l)}}
    \Big),  \\
    & = \sum_{t=0}^T 
    \frac{\partial \mathcal{L}}{\partial \mathbf{h}^{(l)}_{[t]}} 
    \Big(
        \mathbf{s}^{(l)}_{[t]} + 
        \lambda \big( 1 - V_{\text{th}}\frac{\partial \mathbf{s}^{(l)}_{[t-1]}}{\partial \mathbf{h}^{(l)}_{[t-1]}} \big)
        \underbrace{\frac{\partial \mathbf{u}^{(l)}_{[t-1]}}{\partial \mathbf{W}^{(l)}}}_{\substack{\text{unroll} \\ \text{over time}}}
    \Big),  \\
    & = \sum_{t=0}^T 
    \underbrace{\frac{\partial \mathcal{L}}{\partial \mathbf{s}^{(l)}_{[t]}}}_{\substack{\text{gradient from} \\ \text{last layer}}}
    \underbrace{\frac{\partial \mathbf{s}^{(l)}_{[t]}}{\partial \mathbf{h}^{(l)}_{[t]}}}_{\substack{\text{surrogate} \\ \text{gradient}}}
    \bigg( 
        \mathbf{s}_{[t]}^{(l)} + 
        \sum_{k=0}^{t-1} 
        \Big( 
            \prod_{\tau=k}^{t-1} 
            \lambda \big( 
                1 - V_{\text{th}}
                \underbrace{\frac{\partial \mathbf{s}^{(l)}_{[\tau]}}{\partial \mathbf{h}^{(l)}_{[\tau]}}}_{\substack{\text{surrogate} \\ \text{gradient}}}
            \big) 
        \Big) 
        \mathbf{s}^{(l)}_{[k]}
    \bigg) \\
    & \overset{\substack{\text{detach} \\ \text{reset}}}{\approx} \sum_{t=0}^T 
    \frac{\partial \mathcal{L}}{\partial \mathbf{s}^{(l)}_{[t]}} 
    \frac{\partial \mathbf{s}^{(l)}_{[t]}}{\partial \mathbf{h}^{(l)}_{[t]}} 
    \bigg(
        \sum_{k=0}^{t} \lambda^{t-k} \mathbf{s}^{(l)}_{[k]}
    \bigg)
    .
\end{aligned}
\end{equation}
\end{strip}
